# Supplementary material for: Uncertainty quantification by direct propagation of shallow ensembles
Source: arXiv:2402.16621 source file (2024-05-16)
Supplement: Supplementary file 1 [file si.pdf]

# Uncertainty quantification by direct propagation of shallow ensembles

**Supporting Information**

Matthias Kellner[1] and Michele Ceriotti[1, *]

[1] *Laboratory of Computational Science and Modeling, Institut des Matériaux, École Polytechnique Fédérale de Lausanne, 1015 Lausanne, Switzerland*

(Dated: May 14, 2024)

## I. UCI DATASET BENCHMARKS

Table S1 is based on the same experiments as the corresponding table in the main text, but uses the NLL as a metric, for a more direct comparison with previous results in the literature.

We also report (Table S2 and Table S3) a 1:1 comparison of DPOSE (5 ensemble members) with a mean-variance estimator and a mean-variance ensemble (deep ensemble) performed following the same protocol as in Ref. 1, i.e. using a 90:10 train:test split strategy, and no post hoc calibration.

Finally, in Table S4 we demonstrate the convergence of DPOSE estimators with respect to the number of implicit committee members (ie $n_{\text{ens}}$).

| Dataset | MVE | MVEns | **DPOSE** | A | B | C | D | E | F |
|---|---|---|---|---|---|---|---|---|---|
| Training | NLL | NLL | NLL | NLL | NLL | NLL | MSE | MSE | MSE-SS |
| $n_{\text{ens}}$ | - | 5 | 64 | 5 | 5 | 5 | 5 | 5 | 5 |
| Weight sharing | - | no | yes | yes | no | yes | no | no | no |
| Post-hoc cal. | no | no | yes | yes | yes | no | no | yes | yes |
| Housing | $2.63^{\pm0.17}$ | $2.52^{\pm0.17}$ | $2.56^{\pm0.18}$ | $2.89^{\pm0.25}$ | $2.84^{\pm0.27}$ | $2.85^{\pm0.28}$ | $6.22^{\pm3.44}$ | $2.87^{\pm0.56}$ | $2.68^{\pm0.19}$ |
| Concrete | $3.13^{\pm0.19}$ | $3.02^{\pm0.13}$ | $3.05^{\pm0.16}$ | $3.34^{\pm0.21}$ | $3.40^{\pm0.30}$ | $3.36^{\pm0.27}$ | $8.53^{\pm3.28}$ | $3.26^{\pm0.22}$ | $3.26^{\pm0.14}$ |
| Energy | $1.74^{\pm0.16}$ | $1.61^{\pm0.12}$ | $1.58^{\pm0.14}$ | $2.17^{\pm0.15}$ | $2.23^{\pm0.16}$ | $2.37^{\pm0.21}$ | $6.31^{\pm1.62}$ | $2.28^{\pm0.15}$ | $2.31^{\pm0.25}$ |
| Kin8nm | $-1.12^{\pm0.04}$ | $-1.25^{\pm0.02}$ | $-1.15^{\pm0.04}$ | $-1.12^{\pm0.07}$ | $-1.12^{\pm0.07}$ | $-0.58^{\pm0.24}$ | $0.78^{\pm0.53}$ | $-0.98^{\pm0.06}$ | $-0.97^{\pm0.05}$ |
| Naval | $-4.97^{\pm0.33}$ | $-5.11^{\pm0.24}$ | $-4.87^{\pm0.26}$ | $-4.13^{\pm0.32}$ | $-3.88^{\pm0.48}$ | $-3.11^{\pm0.49}$ | $-5.24^{\pm0.20}$ | $-5.31^{\pm0.16}$ | $-5.05^{\pm0.13}$ |
| Power | $2.81^{\pm0.05}$ | $2.79^{\pm0.05}$ | $2.82^{\pm0.04}$ | $2.85^{\pm0.15}$ | $2.86^{\pm0.16}$ | $2.89^{\pm0.12}$ | $26.63^{\pm9.14}$ | $3.07^{\pm0.09}$ | $3.05^{\pm0.06}$ |
| Protein | $2.86^{\pm0.05}$ | $2.82^{\pm0.02}$ | $2.85^{\pm0.05}$ | $2.93^{\pm0.06}$ | $2.93^{\pm0.07}$ | $3.32^{\pm0.46}$ | $32.75^{\pm12.11}$ | $3.27^{\pm0.15}$ | $3.29^{\pm0.07}$ |
| Wine | $1.01^{\pm0.09}$ | $0.94^{\pm0.08}$ | $1.01^{\pm0.16}$ | $1.04^{\pm0.10}$ | $1.09^{\pm0.15}$ | $1.07^{\pm0.15}$ | $13.37^{\pm3.60}$ | $1.18^{\pm0.12}$ | $1.19^{\pm0.13}$ |
| Yacht | $1.94^{\pm0.42}$ | $1.36^{\pm0.21}$ | $1.07^{\pm0.35}$ | $2.00^{\pm0.41}$ | $2.10^{\pm0.36}$ | $2.18^{\pm0.54}$ | $6.70^{\pm6.37}$ | $2.58^{\pm0.75}$ | $2.65^{\pm0.30}$ |
| Years | 3.42 | 3.36 | 3.38 | 3.39 | 3.39 | 3.41 | 29.46 | 3.76 | 3.76 |

TABLE S1. Performance of different UQ approaches, quantified by their negative log likelihood, for a set of regression benchmarks[1, 2]. Standard deviations over multiple train/test splits are shown for each value, except for the larger "years" dataset, for which we use a single split. MVE and MVEns indicate a mean-variance estimator architecture, and a mean-variance deep ensemble; DPOSE indicate the proposed direct propagation of shallow-ensembles approach; models A-F are several variations on a theme for DPOSE, differing by the training target (NLL, or MSE for separate models), by the number of committee members $n_{\text{ens}}$, by the use of weight sharing for all but the last network layer, by the use of post-hoc calibration on a hold-out set.

* michele.ceriotti@epfl.ch

| Dataset | MVE[1] | MVE ours | Deep ens.[1] | Deep ens. ours | DPOSE |
|---|---|---|---|---|---|
| Housing | $2.55^{\pm0.36}$ | $2.68^{\pm0.23}$ | $2.41^{\pm0.25}$ | $2.45^{\pm0.22}$ | $2.84^{\pm0.40}$ |
| Concrete | $3.22^{\pm0.31}$ | $3.11^{\pm0.18}$ | $3.06^{\pm0.18}$ | $2.96^{\pm0.07}$ | $3.01^{\pm0.11}$ |
| Energy | $1.61^{\pm0.40}$ | $1.58^{\pm0.21}$ | $1.38^{\pm0.22}$ | $1.50^{\pm0.11}$ | $1.47^{\pm0.18}$ |
| Kin8nm | $-1.11^{\pm0.04}$ | $-1.14^{\pm0.04}$ | $-1.20^{\pm0.02}$ | $-1.22^{\pm0.02}$ | $-1.15^{\pm0.04}$ |
| Naval | $-5.65^{\pm0.28}$ | $-4.41^{\pm0.99}$ | $-5.63^{\pm0.05}$ | $-4.59^{\pm0.34}$ | $-4.54^{\pm0.56}$ |
| Power | $2.82^{\pm0.04}$ | $2.83^{\pm0.04}$ | $2.79^{\pm0.04}$ | $2.80^{\pm0.04}$ | $2.83^{\pm0.04}$ |
| Protein | $2.87^{\pm0.03}$ | $2.84^{\pm0.03}$ | $2.83^{\pm0.02}$ | $2.81^{\pm0.01}$ | $2.83^{\pm0.03}$ |
| Wine | $1.95^{\pm4.08}$ | $1.04^{\pm0.18}$ | $0.94^{\pm0.12}$ | $0.95^{\pm0.11}$ | $1.06^{\pm0.18}$ |
| Yacht | $1.26^{\pm0.29}$ | $1.87^{\pm0.33}$ | $1.18^{\pm0.21}$ | $1.66^{\pm0.20}$ | $1.03^{\pm0.32}$ |
| Years | 3.41 | 3.47 | 3.35 | 3.35 | 3.38 |

TABLE S2. Comparison of the performance of results (NLL values) from the literature, and those from our equivalent implementation.

| Dataset | MVE[1] | MVE ours | Deep ens.[1] | Deep ens. ours | DPOSE |
|---|---|---|---|---|---|
| Housing | $3.17^{\pm1.00}$ | $3.38^{\pm0.87}$ | $3.28^{\pm1.00}$ | $3.26^{\pm0.94}$ | $3.58^{\pm0.98}$ |
| Concrete | $6.08^{\pm0.56}$ | $5.74^{\pm0.43}$ | $6.03^{\pm0.58}$ | $5.49^{\pm0.35}$ | $5.77^{\pm0.42}$ |
| Energy | $2.11^{\pm0.30}$ | $2.19^{\pm0.23}$ | $2.09^{\pm0.29}$ | $2.19^{\pm0.18}$ | $2.28^{\pm0.24}$ |
| Kin8nm | $0.09^{\pm0.00}$ | $0.09^{\pm0.00}$ | $0.09^{\pm0.00}$ | $0.08^{\pm0.00}$ | $0.08^{\pm0.00}$ |
| Naval | $0.00^{\pm0.00}$ | $0.00^{\pm0.00}$ | $0.00^{\pm0.00}$ | $0.00^{\pm0.00}$ | $0.00^{\pm0.00}$ |
| Power | $4.10^{\pm0.15}$ | $4.11^{\pm0.17}$ | $4.11^{\pm0.17}$ | $4.03^{\pm0.18}$ | $4.13^{\pm0.19}$ |
| Protein | $4.64^{\pm0.01}$ | $4.68^{\pm0.21}$ | $4.71^{\pm0.06}$ | $4.47^{\pm0.07}$ | $4.65^{\pm0.16}$ |
| Wine | $0.64^{\pm0.04}$ | $0.64^{\pm0.04}$ | $0.64^{\pm0.04}$ | $0.63^{\pm0.03}$ | $0.64^{\pm0.03}$ |
| Yacht | $1.43^{\pm0.57}$ | $1.88^{\pm0.55}$ | $1.58^{\pm0.48}$ | $1.58^{\pm0.57}$ | $3.29^{\pm1.79}$ |
| Years | 8.89 | 8.90 | 8.89 | 8.82 | 8.89 |

TABLE S3. Comparison of the performance of results (RMSE values) from the literature, and those from our equivalent implementation.

| Dataset | **DPOSE** | | | | |
|---|---|---|---|---|---|
| Training | NLL | NLL | NLL | NLL | NLL |
| $n_{\text{ens}}$ | 5 | 10 | 16 | 32 | 64 |
| Weight sharing | yes | yes | yes | yes | yes |
| Post-hoc cal. | yes | yes | yes | yes | yes |
| Housing | $-14.14^{\pm41.78}$ | $11.65^{\pm19.47}$ | $10.93^{\pm29.70}$ | $6.75^{\pm21.23}$ | $13.80^{\pm20.05}$ |
| Concrete | $-2.34^{\pm18.39}$ | $17.53^{\pm10.88}$ | $16.65^{\pm9.71}$ | $22.33^{\pm11.07}$ | $18.55^{\pm12.39}$ |
| Energy | $26.58^{\pm9.45}$ | $47.10^{\pm8.84}$ | $50.30^{\pm8.51}$ | $48.94^{\pm11.54}$ | $51.33^{\pm7.80}$ |
| Kin8nm | $13.37^{\pm3.51}$ | $11.88^{\pm3.98}$ | $12.28^{\pm4.16}$ | $12.76^{\pm3.07}$ | $13.50^{\pm4.07}$ |
| Naval | $29.22^{\pm19.33}$ | $29.25^{\pm23.31}$ | $33.61^{\pm12.78}$ | $36.14^{\pm11.72}$ | $43.76^{\pm9.90}$ |
| Power | $-3.05^{\pm15.46}$ | $0.87^{\pm3.24}$ | $1.41^{\pm3.39}$ | $0.99^{\pm2.91}$ | $0.79^{\pm3.24}$ |
| Protein | $6.47^{\pm8.40}$ | $13.15^{\pm5.15}$ | $13.84^{\pm6.00}$ | $14.69^{\pm4.46}$ | $13.21^{\pm5.23}$ |
| Wine | $-8.52^{\pm11.93}$ | $-10.55^{\pm16.08}$ | $-6.46^{\pm14.93}$ | $-9.19^{\pm22.08}$ | $-5.71^{\pm18.52}$ |
| Yacht | $44.68^{\pm22.76}$ | $56.81^{\pm18.62}$ | $55.36^{\pm15.57}$ | $57.14^{\pm12.86}$ | $64.46^{\pm18.61}$ |
| Years | 23.61 | 23.47 | 23.46 | 23.57 | 23.59 |

TABLE S4. Relative Likelihoods of DPOSE predictions with an increasing number of implicit committee members $n_{\text{ens}}$.

## II. CONVERGENCE OF NLL AND CRPS LOSS TRAINING FOR A TOY MODEL

Ref. 3 demonstrates the difficulty in converging the NLL using a test case with a sinusoidal target. We repeat the test comparing NLL and CRPS losses. We sample 1000 uniformly spaced points ($x \in [0, 12]$) from a sinusoidal function (Eq. (S1)) with a homoscedastic noise term $\xi$ which is sampled from a normal distribution with standard deviation $\sigma$ 0.01. We train MLPs (128 neurons and 2 hidden layers using tanh activation functions, using as architectures both mean variance estimators and shallow ensembles) using the NLL and CRPS as training objectives. For reference we also train MLPs, using the MSE loss function as the training objective. We train using mini batch gradient decent using the adam optimizer [4], using a batch size of 100 samples and a fixed learning rate of 5e-04. We construct shallow ensembles with $n_{\text{ens}}$ 64 implicit committee members. We clamp small predicted variances, to a minimum $\varepsilon$ of 1e-8. These parameters are identical to the training procedure of the sinusoidal toy example described in Ref. 3.

$$y(x) = 0.4\,\sin(2\pi x) + \xi, \qquad \xi \sim \mathcal{N}(0,\, \sigma^2 = 0.01^2) \tag{S1}$$

In Fig. S1 we show the loss training curves of mean variance estimators and shallow ensembles trained using the NLL and CRPS training objective. We show the predictions of a shallow ensemble trained using the NLL which has converged to a poor local minimum.

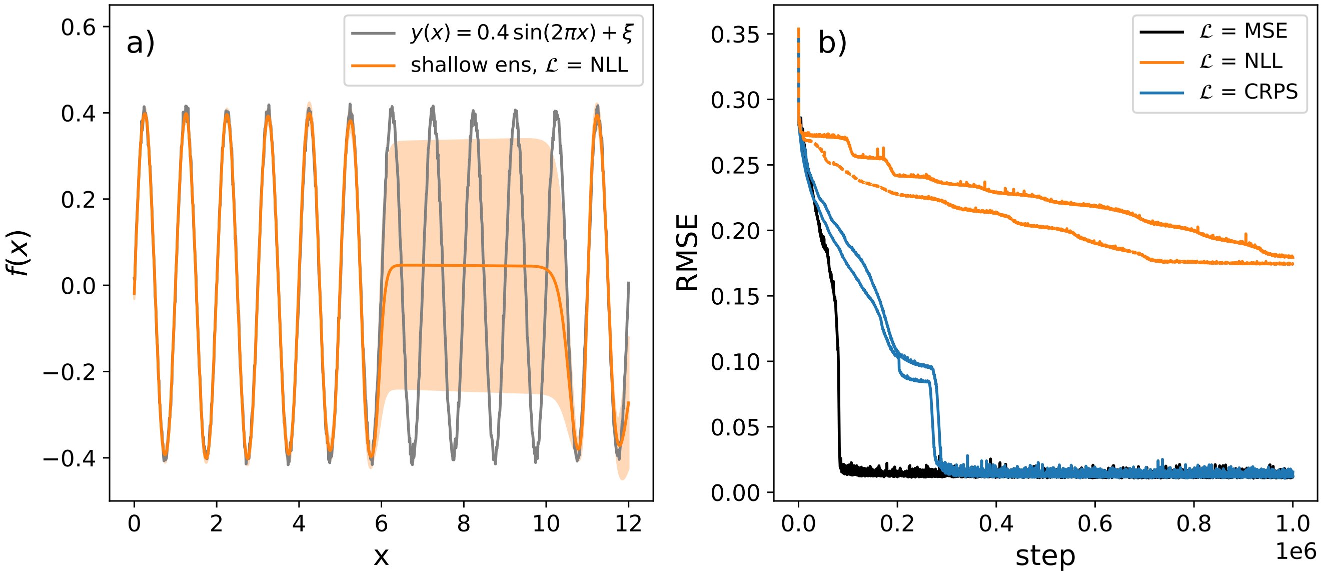


FIG. S1. TBD: (a) toy example and prediction of improperly converged shallow ensemble obtained minimizing the negative log likelihood. (b) training loss curve of Mean Variance estimators and shallow ensembles, minimizing the NLL (orange) or the CRPS (blue). The initial seed for weight initialization is fixed to 0 for this experiment. For reference the training loss curve of an MLP of the same architecture, but with the MSE loss as the training objective is shown.

In Fig. S2 we show training loss curves of shallow ensembles, in which the weights have been initialized with different seeds. We compare again training with the CRPS and NLL objective (5 runs each). We observe similar results as reported in Ref. 3 introducing the $\beta$-NLL objective, that overall the CRPS improves the convergence, yet it is still possible for the estimator to converge to suboptimal local minima.

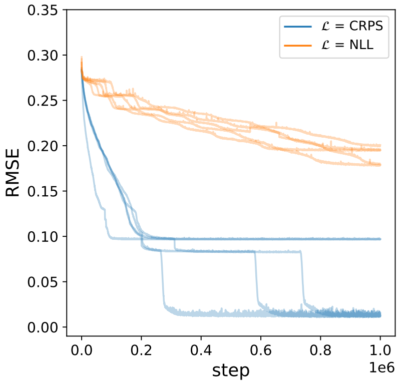


FIG. S2. Loss curves of the sinusoidal toy model, of MLPs initialised with different seed. Blue: shallow ensemble trained with CRPS, orange: shallow ensemble trained with NLL.

## III. PARITY PLOTS OF SHALLOW ENSEMBLE POTENTIALS FOR LARGE LIQUID WATER STRUCTURES

Figure S3 shows the parity plot for the predicted potentials of individual committee members and the mean potential energy estimate with respect to the reference potential energy of a DPOSE estimator for liquid water. The plot shows the predictions and reference potentials for a series of liquid water configurations containing 512 water molecules, sampled at constant temperature and density. We show, as representative examples, the committee member predictions for the committee members 0, 1 and 40 as well as the mean potential, highlighting how individual committee member predictions deviate from the reference potential by a fixed bias across all test structures. It is clear how the mean potential has a constant offset from the parity line (the empirical bias) and how the means of the committee members have each a different constant offset (leading to the ensemble estimate of the bias).

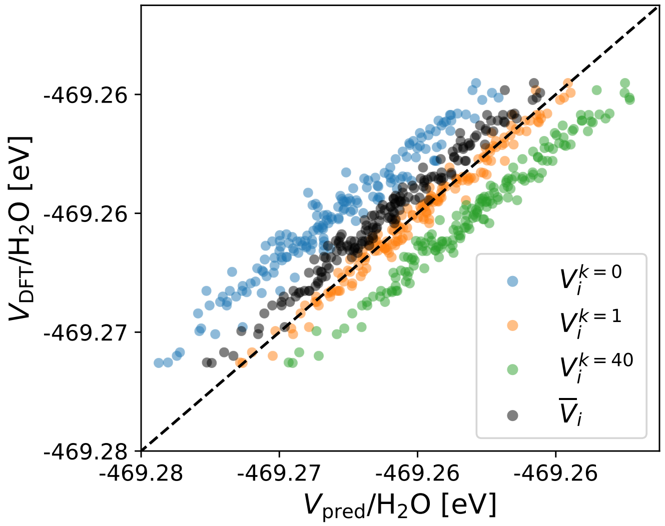


FIG. S3. Parity plots for the potential energy estimates of a DPOSE estimator for liquid water. The parity plot shows predictions and reference potential for liquid water structures containing 512 water molecules at a fixed density. Estimates of committee members $N = 0, 1, 40$ ($V_i^{k=N}$) are plotted as well as the committee mean estimates $\overline{V}_i$.

## IV. CUMULANT EXPANSION APPROXIMATION FOR GAUSSIAN AND NON-GAUSSIAN DISTRIBUTIONS

The cumulant-expansion approximation

$$\langle y \rangle_{V^{(k)}} \approx \langle y \rangle_{\bar{V}} - \beta[\left\langle y(V^{(k)} - \bar{V}) \right\rangle_{\bar{V}} - \langle y \rangle_{\bar{V}} \left\langle V^{(k)} - \bar{V} \right\rangle_{\bar{V}}]. \tag{S2}$$

is based on an expression introduced in Ref. 5 to avoid the difficulties in converging statistical averages during Boltzmann reweighting. The core assumption is that the target quantity and the logarithm of the weighting factor ($y$ and $\beta(V^{(k)} - \bar{V})$ in this case) are approximately distributed as a multivariate Gaussian distribution, which is often the case in atomistic simulation where observables and potential are the result of a combination of multiple weakly-correlated terms. The approximation is usually accurate enough to estimate the uncertainty from ensemble propagation, but it can break down badly if the distribution deviates a lot from a Gaussian. Figure S4 demonstrates a case where the Gaussian assumption is justified - the reweighing of the structural correlations in a simulation of liquid water. Figure S5, instead, shows the issue inherent in the application of the CEA to the calculation of potential fluctuations: the fluctuation term is not Gaussian-distributed, and so it is better to compute the reweighted value using an approximation of the centered moments of $V^{(k)}$.

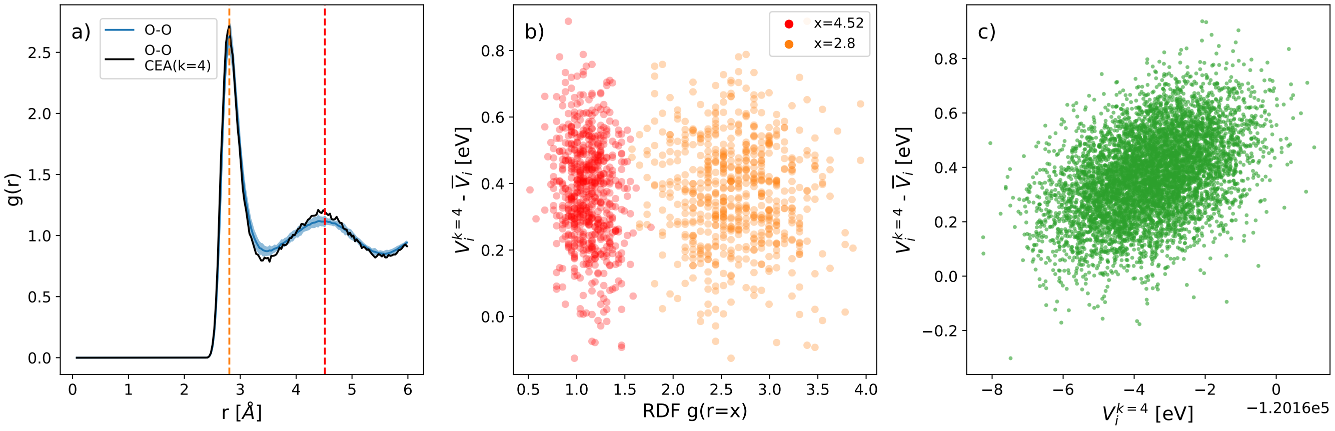


FIG. S4. (a) O-O pair correlation function for a 256-molecule simulation of liquid water at 300K. The black line indicates the reweighted pair correlation function using the potential energy of the committee member $k = 4$, using the cumulant expansion. (b) Correlation of structure-wise ($i$) pair correlation function at 2.80 $\AA$ (orange) and 4.52 $\AA$ (red) with the deviations of the potential energies of committee member $k = 4$, with the mean potential energy of the ensemble $\overline{V}$. (c) Correlation plot of $V^{(k=4)}(A_i)$ and $V^{(k=4)}(A_i) - \bar{V}(A_i)$.

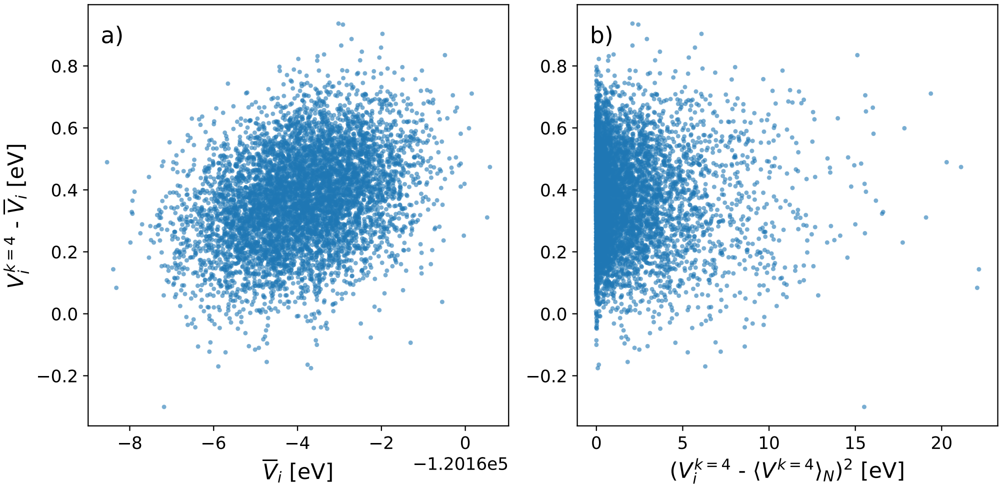


FIG. S5. (a) Correlation plot of $V^{(k=4)}(A_i)$ and $V^{(k=4)}(A_i) - \bar{V}(A_i)$, as in Fig. S4c. (b) Correlation of $V^{(k=4)}(A_i) - \bar{V}(A_i)$ and $(V_i^k - \langle V^k\rangle)^2$. Note that $(V_i^k - \langle V^k\rangle)^2$ is clearly not Gaussian.

## V. PAIR DISTRIBUTION FUNCTION - SUPERCELL-SIZE DEPENDENCY

Fig. S6 shows that using a cumulant expansion approximation avoids the curse of system size in statistical reweighting[5]: when using a non-approximated Boltzmann reweighting the uncertainty of committee members grows exponentially with system size, while the CEA is stable.

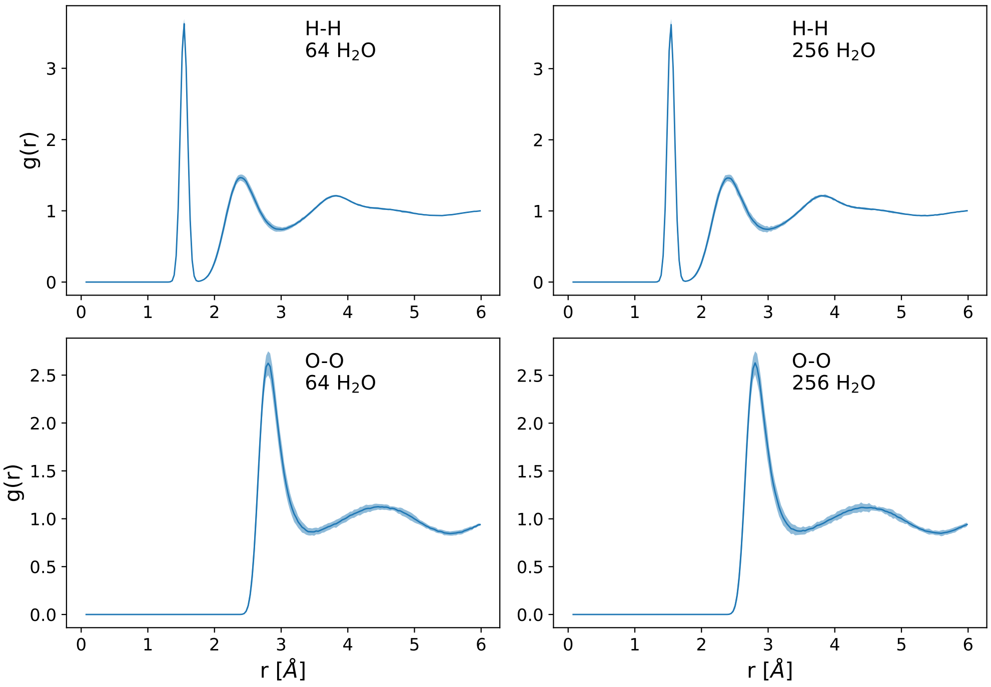


FIG. S6. H-H and O-O pair correlation functions with propagated model uncertainties computed using the CEA. Reweighted pair correlation functions of simulations of 64 water molecules and 256 water molecules reach a good consensus on uncertainty estimates of the $g(r)$.


[1] B. Lakshminarayanan, A. Pritzel, and C. Blundell, Simple and Scalable Predictive Uncertainty Estimation using Deep Ensembles, in *Advances in Neural Information Processing Systems*, Vol. 30, edited by I. Guyon, U. V. Luxburg, S. Bengio, H. Wallach, R. Fergus, S. Vishwanathan, and R. Garnett (Curran Associates, Inc., 2017).

[2] J. M. Hernandez-Lobato and R. Adams, Probabilistic Backpropagation for Scalable Learning of Bayesian Neural Networks, in *Proceedings of the 32nd International Conference on Machine Learning* (PMLR, 2015) pp. 1861–1869.

[3] M. Seitzer, A. Tavakoli, D. Antic, and G. Martius, On the Pitfalls of Heteroscedastic Uncertainty Estimation with Probabilistic Neural Networks, in *International Conference on Learning Representations* (2021).

[4] D. P. Kingma and J. Ba, Adam: A Method for Stochastic Optimization (2017), arxiv:1412.6980 [cs].

[5] M. Ceriotti, G. A. Brain, O. Riordan, and D. E. Manolopoulos, The inefficiency of re-weighted sampling and the curse of system size in high-order path integration, Proc. R. Soc. Math. Phys. Eng. Sci. **468**, 2 (2012).
